# Supplementary material for: SG-Reg: Generalizable and Efficient Scene Graph Registration
Source: arXiv:2504.14440 source file (2025-05-20)
Supplement: Supplementary file 1 [file false_nodes.tex]

\subsubsection{False node matches}
We demonstrated some falsely matched nodes in the 3RScan-Mapping scenes. 

\begin{figure}[h]
    \centering
    \begin{subfigure}[h]{0.4\columnwidth}
       \includegraphics[width=\columnwidth]{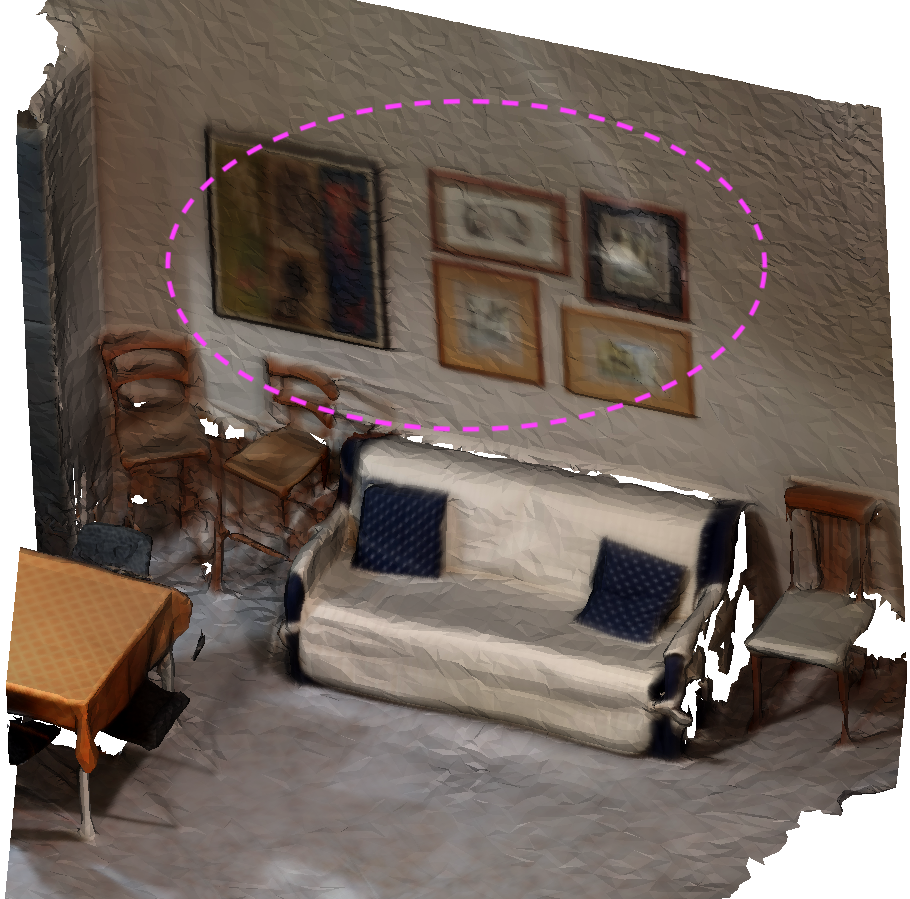}
       \caption{}
    \end{subfigure}
    \begin{subfigure}[h]{0.58\columnwidth}
       \includegraphics[width=\columnwidth]{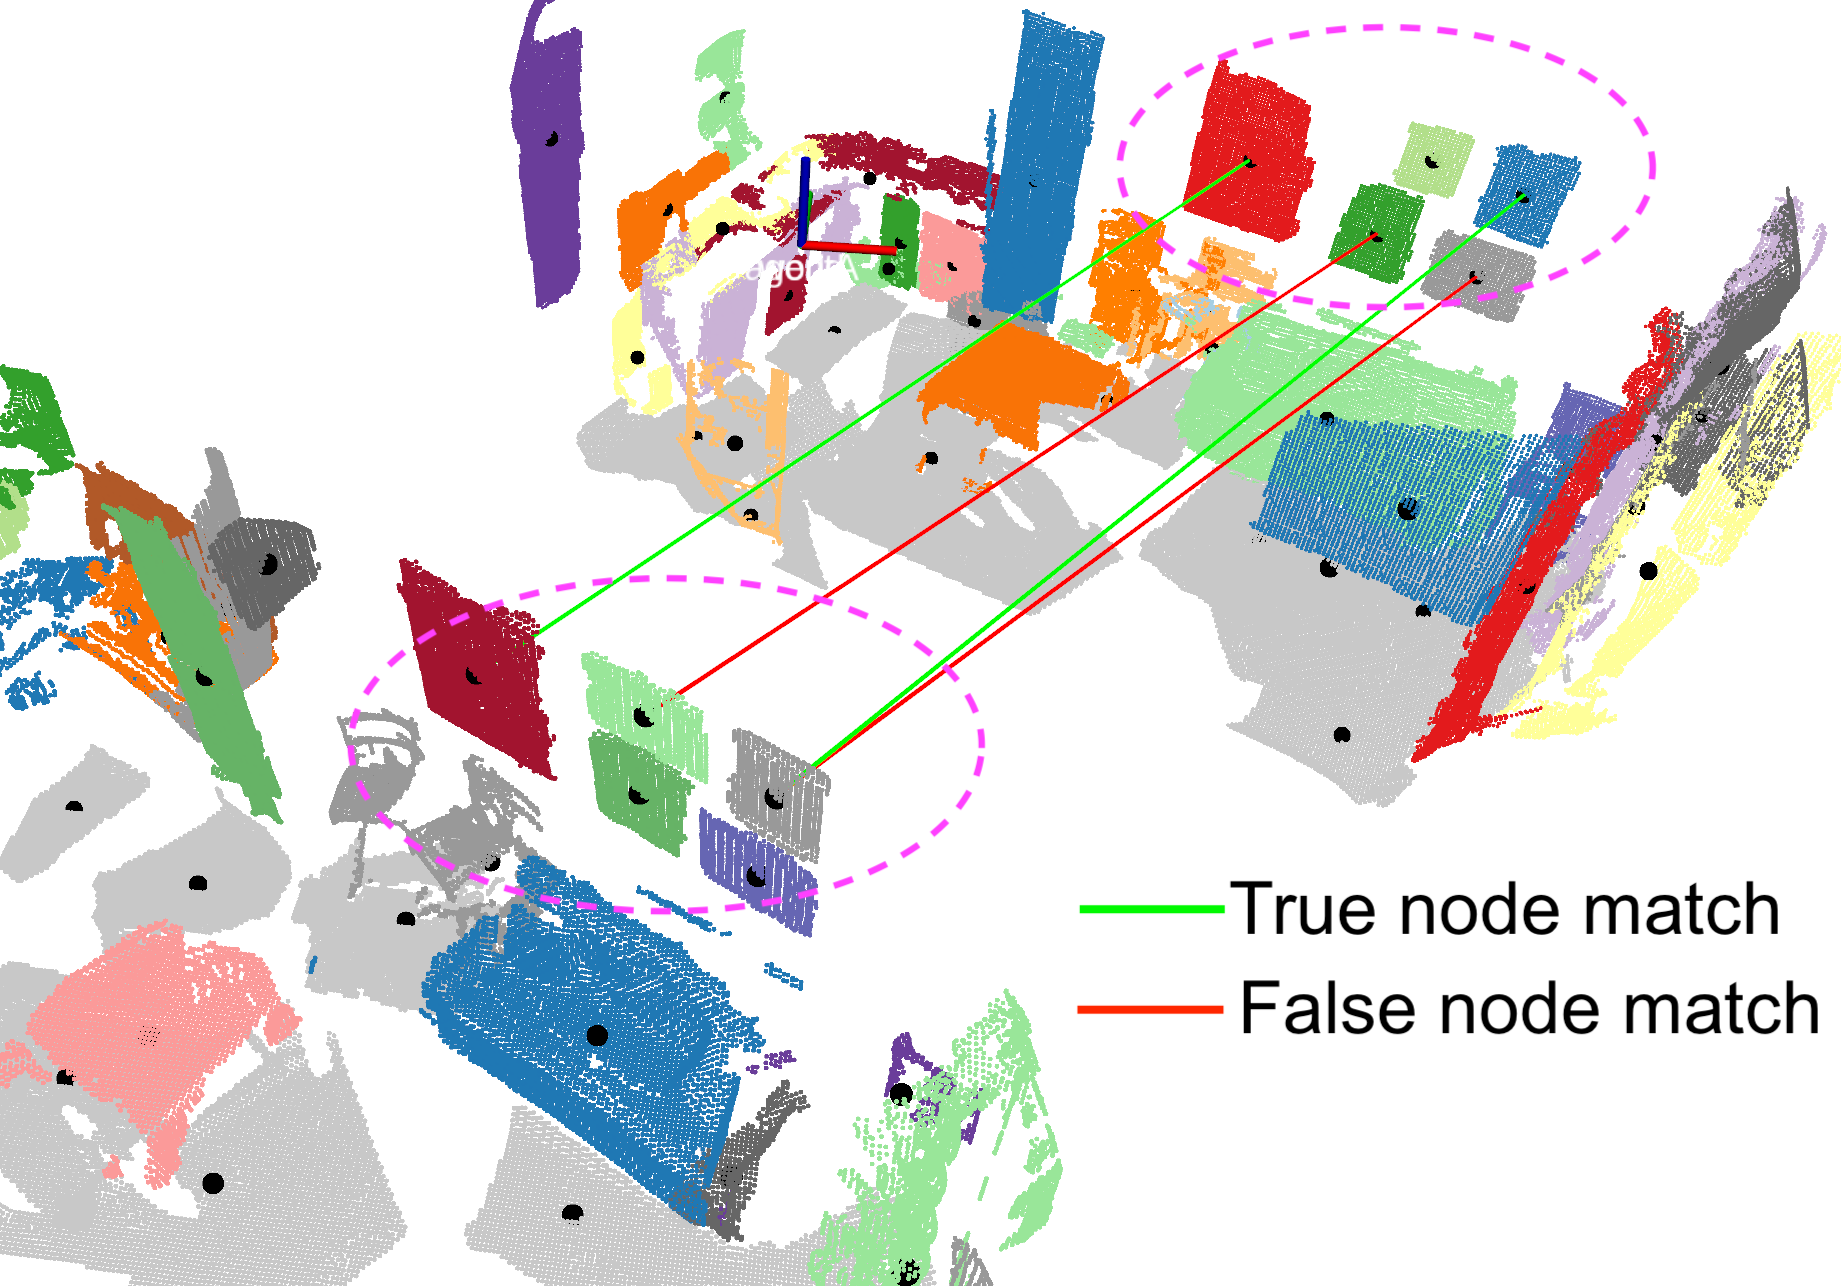}
       \caption{}
    \end{subfigure}
    \caption{A subvolume containing multiple nearby \textit{picture frames}, highlighted by purple circles. The mesh view is shown in (a), while the matching results are presented in (b). Node matches between the \textit{picture frames} in the subvolume.}
    \label{fig:picframes}
\end{figure}
As shown in Fig. \ref{fig:picframes}, the picture frames in the upper row exhibit a closely similar local topology to those in the bottom row. As a result, SG-Reg generates similar node features for both sets, leading to false matches between the two picture frames. To address this issue, one potential solution is to incorporate height information when encoding each semantic node, which would help distinguish the picture frames between the rows.

\begin{figure}
    \centering
   \includegraphics[width=0.9\columnwidth]{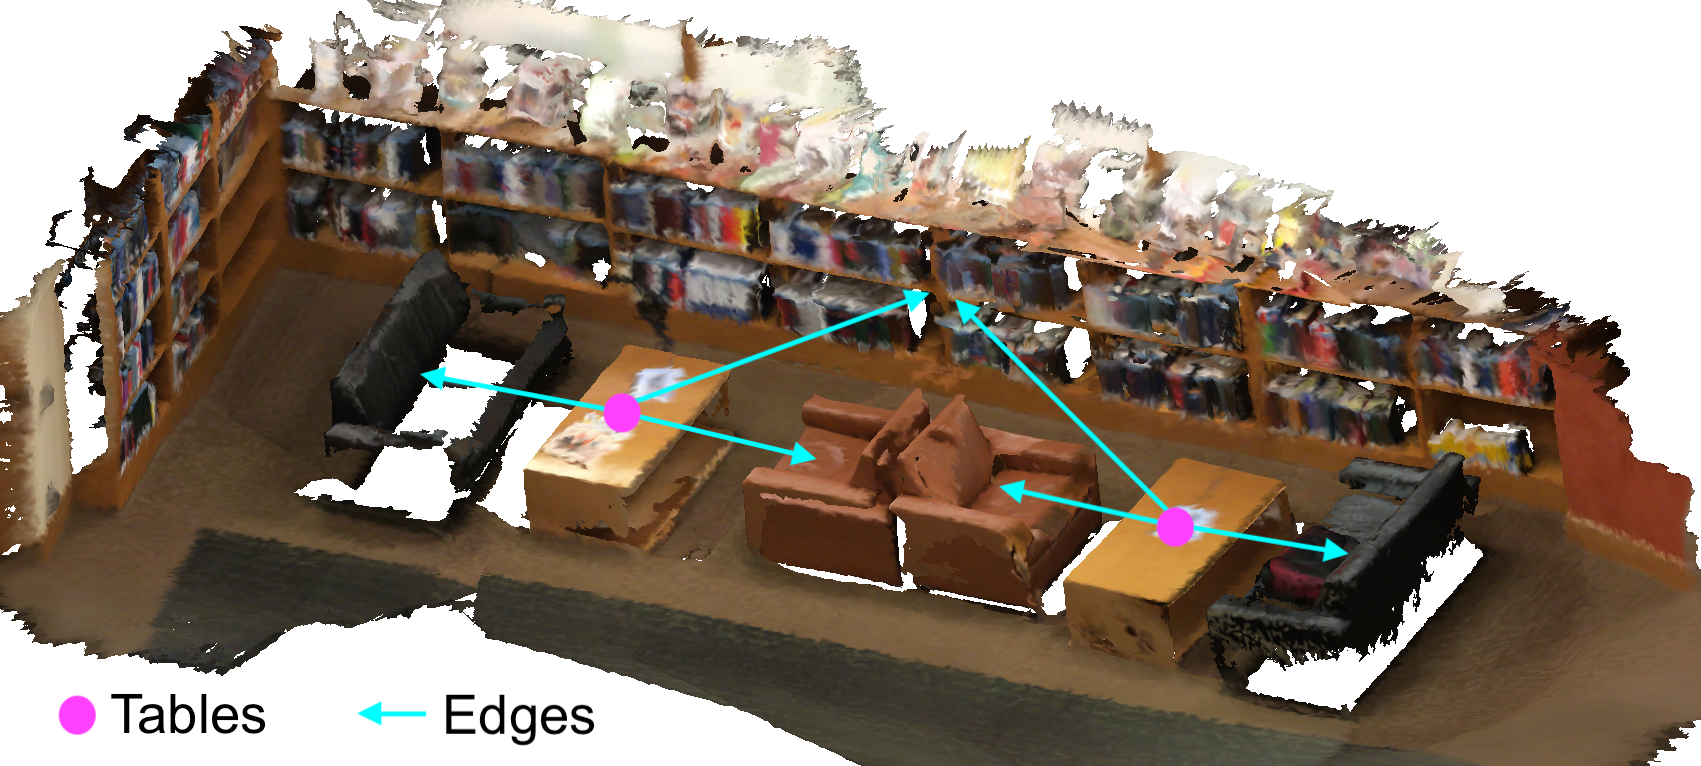}
   \includegraphics[width=\columnwidth]{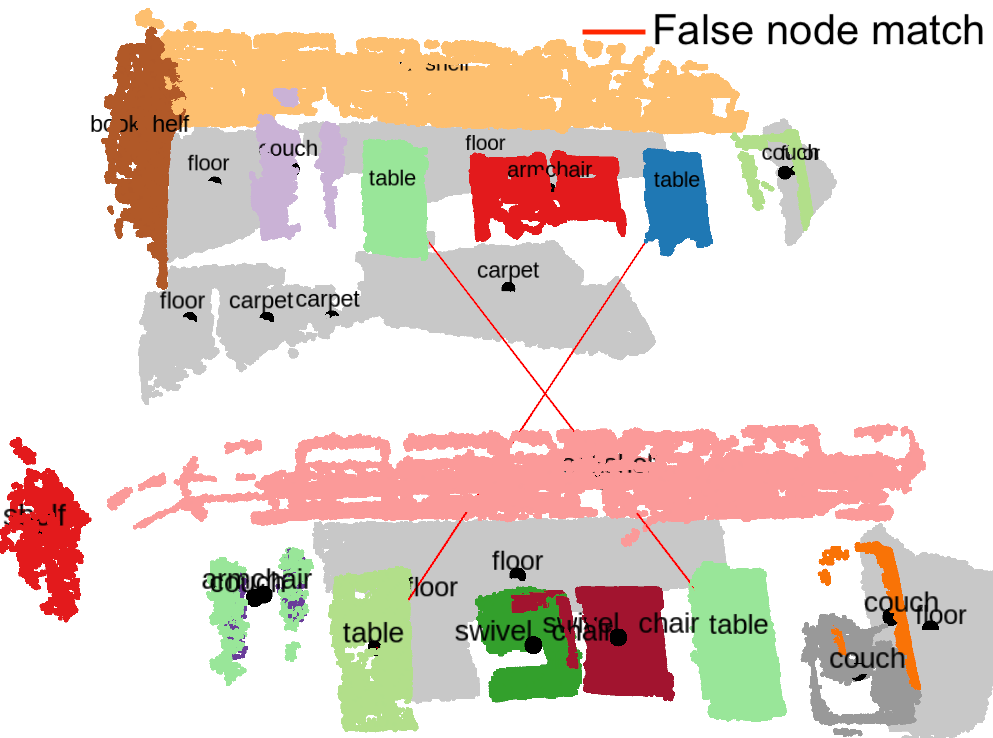}
    \caption{(a) In a ScanNet scene, two tables have closely similar local topology, which are symmetric. Their subvolumes are highlighted in purple circles. (b) SG-Reg falsely matches them.}
    \label{fig:library}
\end{figure}
We present another case of false node matches in Fig. \ref{fig:library}. The local topology and shape of the two tables are nearly identical, leading to ambiguous semantic features. Hence, they are falsely associated. To address this issue, one potential solution is to establish edges between the tables and further objects in the scene, thereby generating semantic node features in a larger perceptual field. It should enable better differentiation of the features of the two tables.
